# Supplementary material for: SpReME: Sparse Regression for Multi-Environment Dynamic Systems
Source: arXiv:2302.05942 source file (2023-03-08)
Supplement: Supplementary file 1 [file appendix.tex]

% %%%%%%%%%%%%%%%%%%%%%%%%%%%%%%%%%%%%%%%%%%%%%%%%%%%%%%%%%%%%%%%%%%%%%%%%%%%%%%%
% %%%%%%%%%%%%%%%%%%%%%%%%%%%%%%%%%%%%%%%%%%%%%%%%%%%%%%%%%%%%%%%%%%%%%%%%%%%%%%%
% % APPENDIX
% %%%%%%%%%%%%%%%%%%%%%%%%%%%%%%%%%%%%%%%%%%%%%%%%%%%%%%%%%%%%%%%%%%%%%%%%%%%%%%%
% %%%%%%%%%%%%%%%%%%%%%%%%%%%%%%%%%%%%%%%%%%%%%%%%%%%%%%%%%%%%%%%%%%%%%%%%%%%%%%%
\newpage
\appendix
\onecolumn
\section{Case study}

As shown in \autoref{table:mask_result}, the Lorenz model has identified incorrect terms in the trained mask. The model identifies three additional terms incorrectly. %The meta-mask trained in the Lorenz dataset leave three extra terms unmasked to compare with the ground truth model.
The dynamics uncovered by the trained mask is as follows:
\begin{align*}
    dx/dt &= \sigma(y-x) + \underline{\epsilon_1 xz^2}, \\
    dy/dt &= x(\rho - z) -y + \underline{\epsilon_2 x^2yz}, \\
    dz/dt &= xy-\beta z + \underline{\epsilon_3 y^2},
\end{align*}
where incorrectly identified terms are the underlined with their coefficient $\epsilon_i$ (c.f., \autoref{eqn:lorenz}).
We find that, at test time, the coefficients of incorrect terms are  small ($<0.00605$), leading to a better performance than the other baseline models.

\begin{figure*}[t!]
    \centering
    \includegraphics[width=\linewidth]{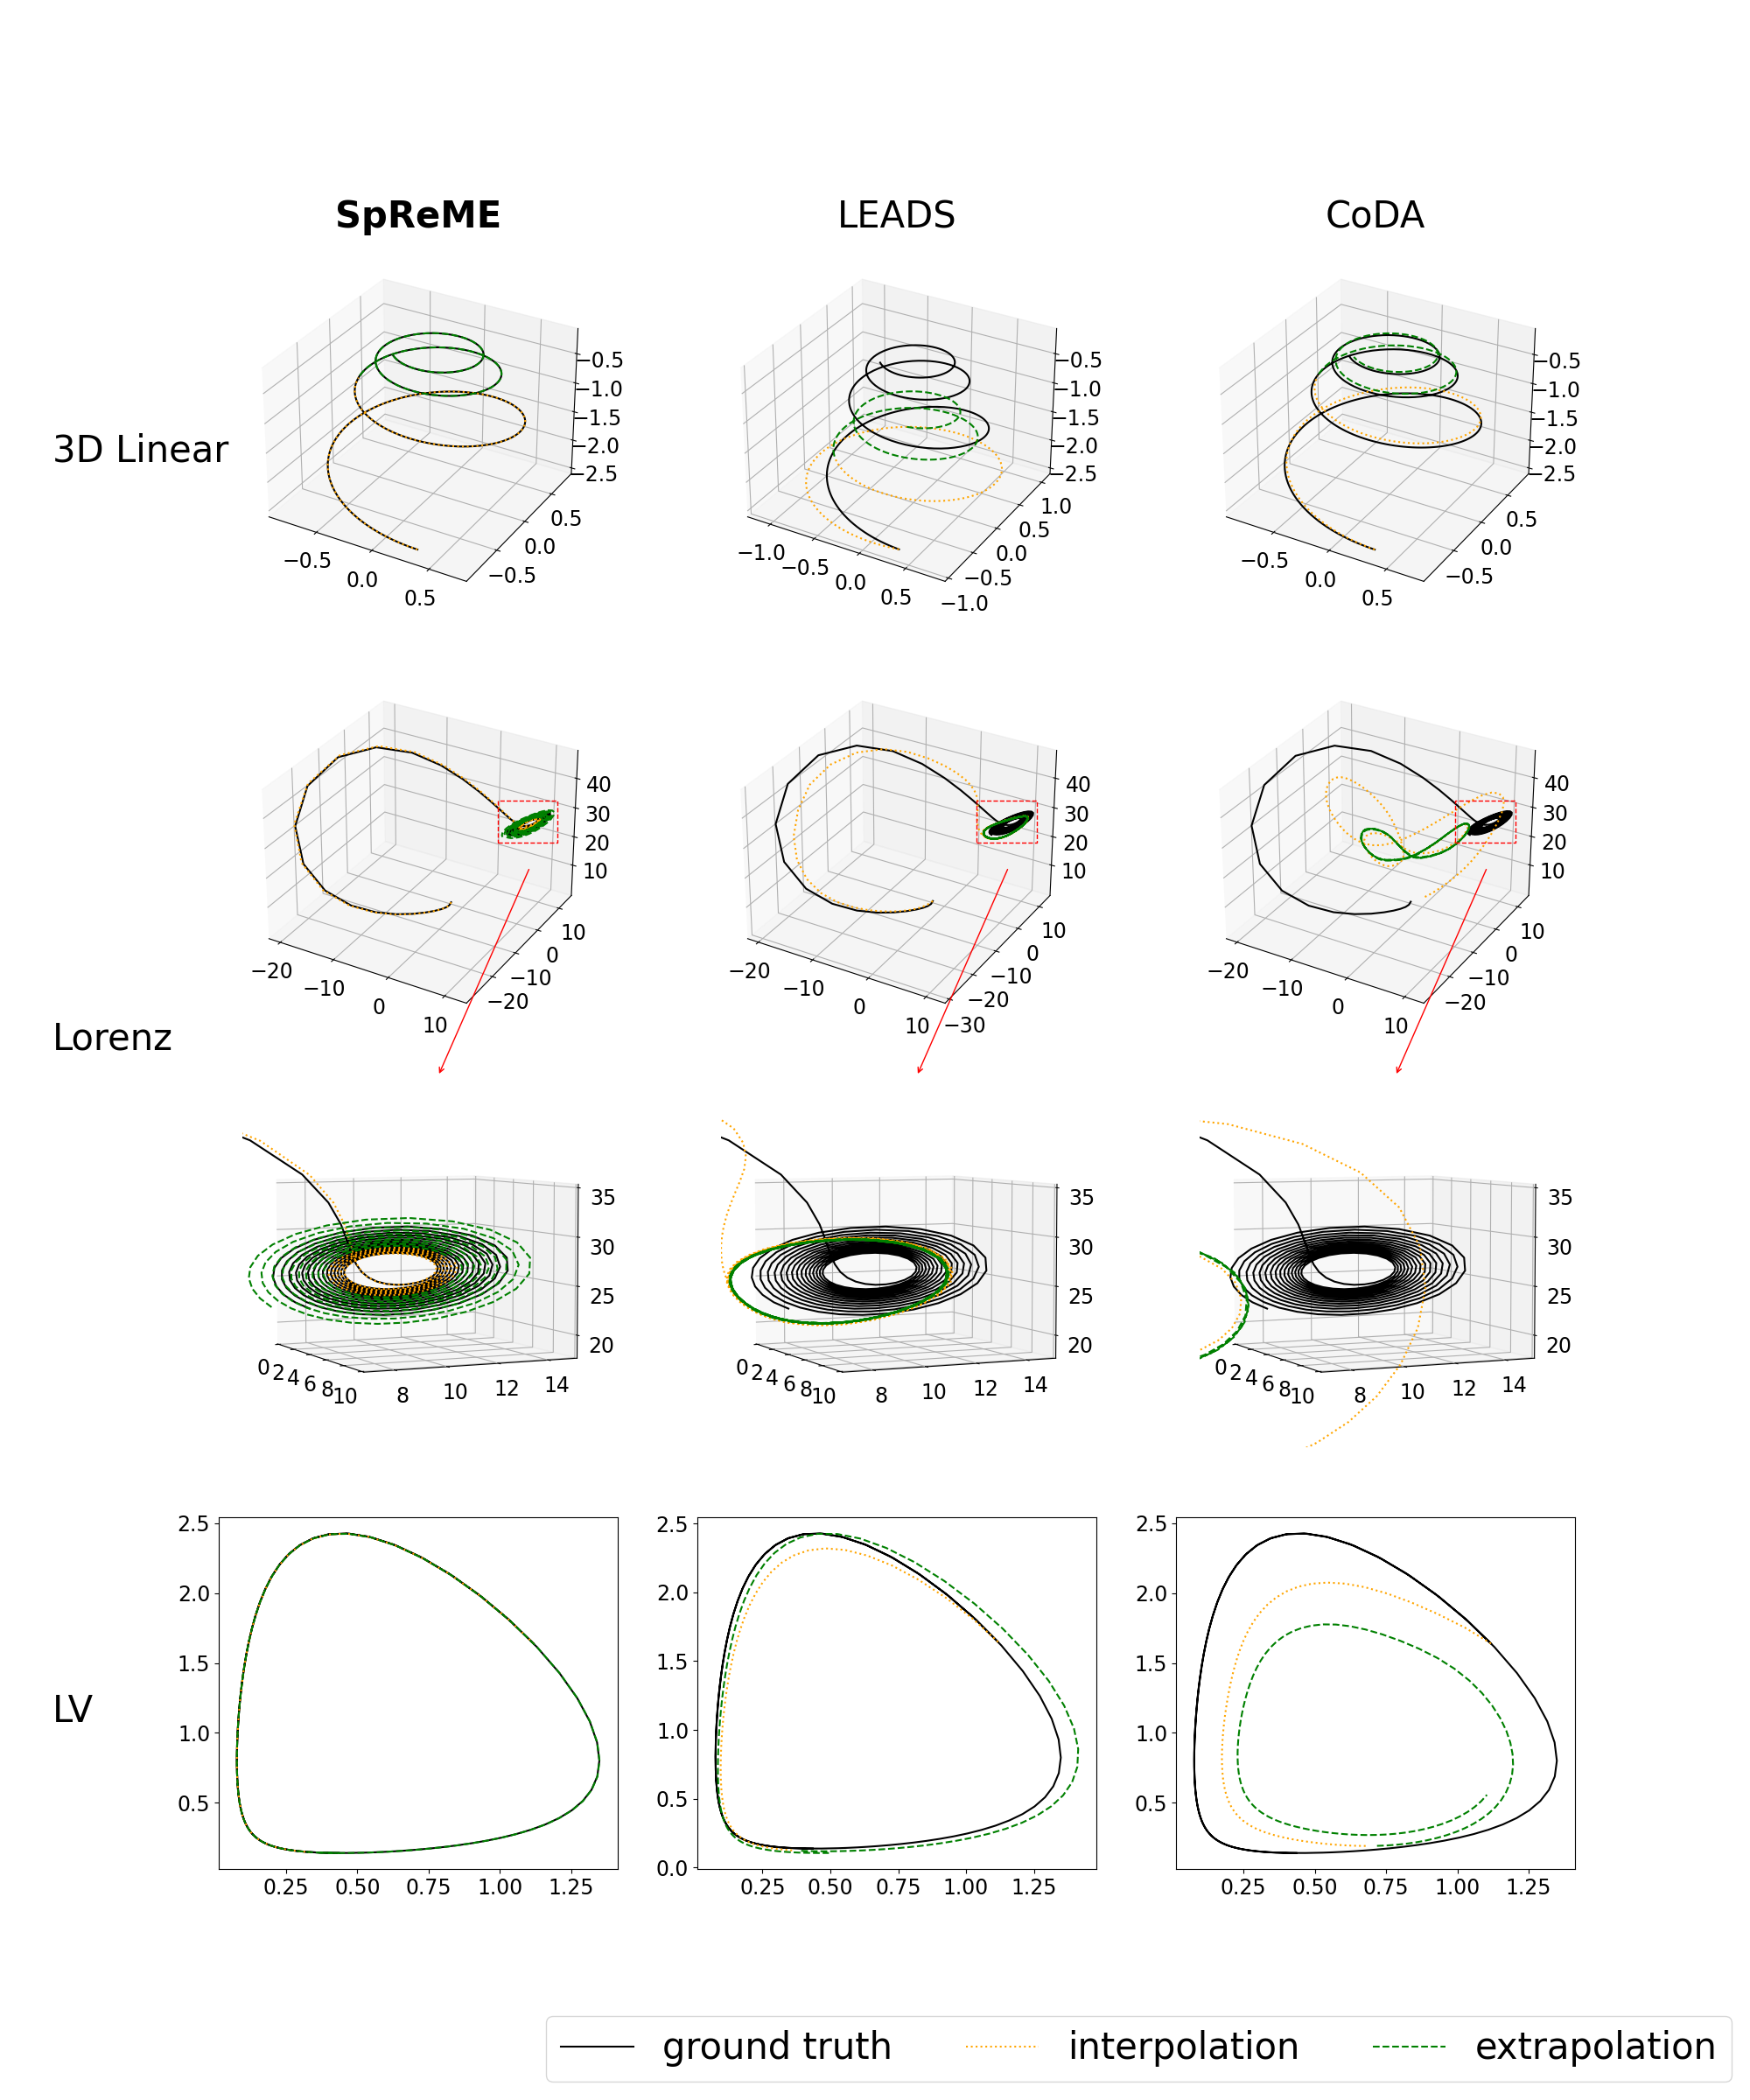}
    \caption{Comparison between the prediction of \ours, LEADS and CoDA for 3D linear, Lorenz and Lotka-Volterra models. The solid black lines are ground truth, the dotted orange lines are interpolation results, and the dashed green lines are extrapolation results. With the Lorenz model, we provide the enlarged views of the extrapolated region (red boxed), changing dramatically from the training trajectory.}
    \label{fig:results}
    \vspace{1em}
\end{figure*}
